# Supplementary material for: Towards Compatible Fine-tuning for Vision-Language Model Updates
Source: arXiv:2412.20895 source file (2024-12-30)
Supplement: Supplementary file 1 [file appendix.tex]

\clearpage
\appendix

%%%%%%%%%%
\section{Further xx}
\label{sec:appendix_xx}
